# Supplementary material for: Emergence of highly coherent quantum subsystems of a noisy and dense spin system
Source: arXiv:2210.01024 source file (2024-01-17)
Supplement: Supplementary file 1 [file Parameters.tex]

% Optical absorption measurements by the manufacturer at 487\,nm yielded $0.1\%$ and $0.004\%$ respectively. Rutherford backscattering confirmed the $x=0.09\pm0.002\%$ for the denser sample.


%%%%%%%%%%%%%%%%%%%%%%%%%%%%%%%%%%%%%%%%%%%%%%%%%%%%%%
%%%%%%%%%%%%%%%%%%%%%%%%%%%%%%%%%%%%%%%%%%%%%%%%%%%%%%
% Pulse configurations
%%%%%%%%%%%%%%%%%%%%%%%%%%%%%%%%%%%%%%%%%%%%%%%%%%%%%%
%%%%%%%%%%%%%%%%%%%%%%%%%%%%%%%%%%%%%%%%%%%%%%%%%%%%%%

%%%%%%%%%%%%%%%
% B=38mT wide range frEq.scan 50MHz res.
%%%%%%%%%%%%%%%
% name	type	t	tp	scale	nu_init	channel	A_n	x_n	deltax_n	Qshift	phase
% pi/2	Gausscascade	0.	100.	0.244	1.5	3.	1.	0.5	0.4	0.0161	0.
% pi	Gausscascade	500.	200.	0.244	1.5	3.	1.	0.5	0.4	0.0161	0.
% det	1200.	1024.	1.5								
% digrate	2.										

% freq	B	reptime	shots	avgs	Ntot	IFgain	IFgain_levels
% 26.	380.	1.*10^6	20.	1.	80.	1.	{1.,18.7115,36.1442}

%%%%%%%%%%%%%%%
% B=38mT narrow range freq.scan around minimum 10MHz res.
%%%%%%%%%%%%%%%
% name	type	t	tp	scale	nu_init	channel	A_n	x_n	deltax_n	Qshift	phase
% pi/2	Gausscascade	0.	100.	0.03	1.5	3.	1.	0.5	0.4	0.0161	0.
% pi	Gausscascade	300.	200.	0.03	1.5	3.	1.	0.5	0.4	0.0161	0.
% det	800.	1024.	1.5								
% digrate	2.										


% freq	B	reptime	shots	avgs	Ntot	IFgain	IFgain_levels
% 35.53	380.	2.*10^6	200.	1.	1980.	1.	{1.,18.7115,36.1442}





%%%%%%%%%%%%%%%
% B=0mT wide range frEq.scan 50MHz res. (currently appendix?)
%%%%%%%%%%%%%%%
% name	type	t	tp	scale	nu_init	channel	A_n	x_n	deltax_n	Qshift	phase
% pi/2	Gausscascade	0.	100.	0.244	1.5	3.	1.	0.5	0.4	0.0161	0.
% pi	Gausscascade	500.	200.	0.244	1.5	3.	1.	0.5	0.4	0.0161	0.
% det	1200.	1024.	1.5								
% digrate	2.										

% freq	B	reptime	shots	avgs	Ntot	IFgain	IFgain_levels
% 26.	4.	1.*10^6	50.	1.	30.	2.	{1.,18.7115,36.1442}


%%%%%%%%%%%%%%%
% B=38mT nnn pair peak
%%%%%%%%%%%%%%%
% name	type	t	tp	scale	nu_init	channel	A_n	x_n	deltax_n	Qshift	phase
% pi/2	Gausscascade	0.	100.	0.03	1.5	3.	1.	0.5	0.4	0.0161	0.
% pi	Gausscascade	500.	200.	0.03	1.5	3.	1.	0.5	0.4	0.0161	0.
% det	1200.	1024.	1.5								
% digrate	2.										

% freq	B	reptime	shots	avgs	Ntot	IFgain	IFgain_levels
% 35.53	380.	2.*10^6	200.	1.	41.	1.	{1.,18.7115,36.1442}



%%%%%%%%%%%%%%%
% B=0mT AF and FM nn and nnn pair peaks
%%%%%%%%%%%%%%%
% name	type	t	tp	scale	nu_init	channel	A_n	x_n	deltax_n	Qshift	phase
% pi/2	Gausscascade	0.	100.	0.014	1.5	3.	1.	0.5	0.4	0.0161	0.
% pi	Gausscascade	500.	200.	0.014	1.5	3.	1.	0.5	0.4	0.0161	0.
% det	1200.	1024.	1.5								
% digrate	2.										

% freq	B	reptime	shots	avgs	Ntot	IFgain	IFgain_levels
% 36.97	4.	2.*10^6	200.	1.	41.	1.	{1.,18.7115,36.1442}

% name	type	t	tp	scale	nu_init	channel	A_n	x_n	deltax_n	Qshift	phase
% pi/2	Gausscascade	0.	100.	0.014	1.5	3.	1.	0.5	0.4	0.0161	0.
% pi	Gausscascade	500.	200.	0.014	1.5	3.	1.	0.5	0.4	0.0161	0.
% det	1200.	1024.	1.5								
% digrate	2.										

% freq	B	reptime	shots	avgs	Ntot	IFgain	IFgain_levels
% 36.54	4.	2.*10^6	200.	1.	41.	1.	{1.,18.7115,36.1442}

% name	type	t	tp	scale	nu_init	channel	A_n	x_n	deltax_n	Qshift	phase
% pi/2	Gausscascade	0.	100.	0.027	1.5	3.	1.	0.5	0.4	0.0161	0.
% pi	Gausscascade	500.	200.	0.027	1.5	3.	1.	0.5	0.4	0.0161	0.
% det	1200.	1024.	1.5								
% digrate	2.										

% freq	B	reptime	shots	avgs	Ntot	IFgain	IFgain_levels
% 35.8	4.	2.*10^6	200.	1.	41.	1.	{1.,18.7115,36.1442}

% name	type	t	tp	scale	nu_init	channel	A_n	x_n	deltax_n	Qshift	phase
% pi/2	Gausscascade	0.	100.	0.029	1.5	3.	1.	0.5	0.4	0.0161	0.
% pi	Gausscascade	500.	200.	0.029	1.5	3.	1.	0.5	0.4	0.0161	0.
% det	1200.	1024.	1.5								
% digrate	2.										

% freq	B	reptime	shots	avgs	Ntot	IFgain	IFgain_levels
% 35.44	4.	2.*10^6	200.	1.	41.	1.	{1.,18.7115,36.1442}

%%%%%%%%%%%%%%%
% B=38mT x=0.1% envelopes as fct. of frEq. (Fig 3 a)
%%%%%%%%%%%%%%%
% name	type	t	tp	scale	nu_init	channel	A_n	x_n	deltax_n	Qshift	phase
% pi/2	Gausscascade	0.	100.	0.184	1.5	3.	1.	0.5	0.4	0.0161	0.
% pi	Gausscascade	500.	200.	0.184	1.5	3.	1.	0.5	0.4	0.0161	0.
% det	1200.	1024.	1.5								
% digrate	2.										


% freq	B	reptime	shots	avgs	Ntot	IFgain	IFgain_levels
% 27.04	380.	1.*10^6	20.	1.	200.	0.	{1.,18.7115,36.1442}


%%%%%%%%%%%%%%%
% B=38mT x=0.01% main peak frEq.sweep (Fig 3 e inset)
%%%%%%%%%%%%%%%
% name	type	t	tp	scale	nu_init	channel	A_n	x_n	deltax_n	Qshift	phase
% pi/2	chirp	0.	100.	0.18	1.5	3.	 - 	 - 	 - 	0.0161	0.
% pi	chirp	1000.	200.	0.18	1.5	3.	 - 	 - 	 - 	0.0161	0.
% det	2200.	8192.	1.5								
% digrate	2.										


% freq	B	reptime	shots	avgs	Ntot	IFgain	IFgain_levels
% 27.8	380.	2.*10^6	100.	1.	151.	1.	{1.,18.7115,36.1442}

%%%%%%%%%%%%%%%
% B=38mT x=0.01% envelopes as fct. of frEq. (Fig 3 e)
%%%%%%%%%%%%%%%

% name	type	t	tp	scale	nu_init	channel	A_n	x_n	deltax_n	Qshift	phase
% pi/2	chirp	0.	25.	0.15	1.5	3.	 - 	 - 	 - 	0.0161	0.
% pi	chirp	400.	50.	0.15	1.5	3.	 - 	 - 	 - 	0.0161	0.
% det	850.	2048.	1.5								
% digrate	2.										

% freq	B	reptime	shots	avgs	Ntot	IFgain	IFgain_levels
% 27.89	380.	2.*10^6	100.	1.	25500.	0.	{1.,18.7115,36.1442}

%%%%%%%%%%%%%%%
% B=38mT x=0.1%iso High SNR traces Main peak and side
%%%%%%%%%%%%%%%
% Main
% name	type	t	tp	scale	nu_init	channel	A_n	x_n	deltax_n	Qshift	phase
% pi/2	Gausscascade	0.	100.	0.27	1.5	3.	1.	0.5	0.4	0.0161	0.
% pi	Gausscascade	350.	200.	0.27	1.5	3.	1.	0.5	0.4	0.0161	0.
% det	900.	2048.	1.5								
% freq	B	reptime	shots	avgs	Ntot	IFgain	IFgain_levels
% 27.8	379.	2.*10^6	100.	10.	100.	2.	{1.,18.7115,36.1442}

% Main side
% name	type	t	tp	scale	nu_init	channel	A_n	x_n	deltax_n	Qshift	phase
% pi/2	Gausscascade	0.	100.	0.24	1.5	3.	1.	0.5	0.4	0.0161	0.
% pi	Gausscascade	350.	200.	0.24	1.5	3.	1.	0.5	0.4	0.0161	0.
% det	900.	2048.	1.5								
% freq	B	reptime	shots	avgs	Ntot	IFgain	IFgain_levels
% 27.98	379.	2.*10^6	100.	10.	100.	2.	{1.,18.7115,36.1442}

%%%%%%%%%%%%%%%
% B=38mT x=0.1%iso High SNR trace NNN pair peak 100/200ns pulses
%%%%%%%%%%%%%%%
% name	type	t	tp	scale	nu_init	channel	A_n	x_n	deltax_n	Qshift	phase
% pi/2	Gausscascade	0.	100.	0.005	1.5	3.	1.	0.5	0.4	0.0161	0.
% pi	Gausscascade	350.	200.	0.005	1.5	3.	1.	0.5	0.4	0.0161	0.
% det	900.	2048.	1.5								


% freq	B	reptime	shots	avgs	Ntot	IFgain	IFgain_levels
% 35.535	379.	2.*10^6	100.	10.	100.	2.	{1.,18.7115,36.1442}

%%%%%%%%%%%%%%%
% B=38mT x=0.1%iso High SNR trace NNN pair peak 10/20ns pulses
%%%%%%%%%%%%%%%
% name	type	t	tp	scale	nu_init	channel	A_n	x_n	deltax_n	Qshift	phase
% pi/2	Gausscascade	0.	10.	0.05	1.5	3.	1.	0.5	0.4	0.0161	0.
% pi	Gausscascade	280.	20.	0.05	1.5	3.	1.	0.5	0.4	0.0161	0.
% det	580.	2048.	1.5								
% freq	B	reptime	shots	avgs	Ntot	IFgain	IFgain_levels
% 35.535	379.	2.*10^6	100.	10.	100.	0.	{1.,18.7115,36.1442}

%%%%%%%%%%%%%%%
% B=0mT x=0.1%iso High SNR trace "main"
%%%%%%%%%%%%%%%

% name	type	t	tp	scale	nu_init	channel	A_n	x_n	deltax_n	Qshift	phase
% pi/2	Gausscascade	0.	20.	0.77	1.5	3.	1.	0.5	0.4	0.0161	0.
% pi	Gausscascade	280.	40.	0.77	1.5	3.	1.	0.5	0.4	0.0161	0.
% det	600.	2048.	1.5								

% freq	B	reptime	shots	avgs	Ntot	IFgain	IFgain_levels
% 28.26	0.	2.*10^6	100.	20.	50.	2.	{1.,18.7115,36.1442}

%%%%%%%%%%%%%%%
% B=0mT x=0.1%iso High SNR trace FM NNN peak
%%%%%%%%%%%%%%%
% name	type	t	tp	scale	nu_init	channel	A_n	x_n	deltax_n	Qshift	phase
% pi/2	Gausscascade	0.	10.	0.39	1.5	3.	1.	0.5	0.4	0.0161	0.
% pi	Gausscascade	280.	20.	0.39	1.5	3.	1.	0.5	0.4	0.0161	0.
% det	580.	2048.	1.5								

% freq	B	reptime	shots	avgs	Ntot	IFgain	IFgain_levels
% 35.425	0.	2.*10^6	100.	20.	50.	1.	{1.,18.7115,36.1442}

%%%%%%%%%%%%%%%
% B=0mT x=0.1%iso High SNR trace AF NNN peak
%%%%%%%%%%%%%%%
% name	type	t	tp	scale	nu_init	channel	A_n	x_n	deltax_n	Qshift	phase
% pi/2	Gausscascade	0.	10.	0.39	1.5	3.	1.	0.5	0.4	0.0161	0.
% pi	Gausscascade	280.	20.	0.39	1.5	3.	1.	0.5	0.4	0.0161	0.
% det	580.	2048.	1.5								

% freq	B	reptime	shots	avgs	Ntot	IFgain	IFgain_levels
% 35.825	0.	2.*10^6	100.	20.	50.	1.	{1.,18.7115,36.1442}

%%%%%%%%%%%%%%%
% CPMG B=38mT x=0.1%iso Main peak
%%%%%%%%%%%%%%%
% name	type	t	tp	scale	nu_init	channel	A_n	x_n	deltax_n	Qshift	phase
% pi/2	chirp	0.	20.	0.58	1.5	3.	 - 	 - 	 - 	0.0161	0.
% pi	chirp	270.	40.	0.58	1.5	3.	 - 	 - 	 - 	0.0161	0.
% det	550.	1024.	1.5								
% digrate	2.										

% freq	B	reptime	shots	avgs	Ntot	IFgain	IFgain_levels
% 27.8	379.	2.*10^6	10.	1.	1920.	2.	{1.,18.7115,36.1442}

%%%%%%%%%%%%%%%
% CPMG B=38mT x=0.1%iso NNN pair peak
%%%%%%%%%%%%%%%

% name	type	t	tp	scale	nu_init	channel	A_n	x_n	deltax_n	Qshift	phase
% pi/2	chirp	0.	2.	0.11	1.5	3.	 - 	 - 	 - 	0.0161	0.
% pi	chirp	279.	4.	0.11	1.5	3.	 - 	 - 	 - 	0.0161	0.
% det	559.	1024.	1.5								
% digrate	2.										

% freq	B	reptime	shots	avgs	Ntot	IFgain	IFgain_levels
% 35.535	379.	2.*10^6	20.	1.	1920.	0.	{1.,18.7115,36.1442}

%%%%%%%%%%%%%%%
% Appendix
%%%%%%%%%%%%%%%

%%%%%%%%%%%%%%%
% All four "butterfly" measurements of 0.01%iso around B=0
%%%%%%%%%%%%%%%

% name	type	t	tp	scale	nu_init	channel	A_n	x_n	deltax_n	Qshift	phase
% pi/2	chirp	0.	100.	0.13	1.5	3.	Missing[KeyAbsent,A_n1]	Missing[KeyAbsent,x_n1]	Missing[KeyAbsent,deltax_n1]	0.0161	0.
% pi	chirp	400.	200.	0.13	1.5	3.	Missing[KeyAbsent,A_n2]	Missing[KeyAbsent,x_n2]	Missing[KeyAbsent,deltax_n2]	0.0161	0.
% det	1000.	2048.	1.5								
% digrate	2.										


% freq	B	reptime	shots	avgs	Ntot	IFgain	IFgain_levels
% 28.05	2.	2.*10^6	200.	1.	1176.	0.	{1.,18.7115,36.1442}


% name	type	t	tp	scale	nu_init	channel	A_n	x_n	deltax_n	Qshift	phase
% pi/2	chirp	0.	100.	0.13	1.5	3.	Missing[KeyAbsent,A_n1]	Missing[KeyAbsent,x_n1]	Missing[KeyAbsent,deltax_n1]	0.0161	0.
% pi	chirp	400.	200.	0.13	1.5	3.	Missing[KeyAbsent,A_n2]	Missing[KeyAbsent,x_n2]	Missing[KeyAbsent,deltax_n2]	0.0161	0.
% det	1000.	2048.	1.5								
% digrate	2.										


% freq	B	reptime	shots	avgs	Ntot	IFgain	IFgain_levels
% 28.05	9.	2.*10^6	200.	1.	2296.	0.	{1.,18.7115,36.1442}


% name	type	t	tp	scale	nu_init	channel	A_n	x_n	deltax_n	Qshift	phase
% pi/2	chirp	0.	100.	0.13	1.5	3.	Missing[KeyAbsent,A_n1]	Missing[KeyAbsent,x_n1]	Missing[KeyAbsent,deltax_n1]	0.0161	0.
% pi	chirp	400.	200.	0.13	1.5	3.	Missing[KeyAbsent,A_n2]	Missing[KeyAbsent,x_n2]	Missing[KeyAbsent,deltax_n2]	0.0161	0.
% det	1000.	2048.	1.5								
% digrate	2.										


% freq	B	reptime	shots	avgs	Ntot	IFgain	IFgain_levels
% 28.05	24.	2.*10^6	200.	1.	3416.	0.	{1.,18.7115,36.1442}


% name	type	t	tp	scale	nu_init	channel	A_n	x_n	deltax_n	Qshift	phase
% pi/2	chirp	0.	100.	0.04	1.5	3.	Missing[KeyAbsent,A_n1]	Missing[KeyAbsent,x_n1]	Missing[KeyAbsent,deltax_n1]	0.0161	0.
% pi	chirp	400.	200.	0.04	1.5	3.	Missing[KeyAbsent,A_n2]	Missing[KeyAbsent,x_n2]	Missing[KeyAbsent,deltax_n2]	0.0161	0.
% det	1000.	2048.	1.5								
% digrate	2.										


% freq	B	reptime	shots	avgs	Ntot	IFgain	IFgain_levels
% 29.425	2.	2.*10^6	200.	1.	3416.	0.	{1.,18.7115,36.1442}
